# Supplementary material for: Semantic View Synthesis
Source: arXiv:2008.10598 source file (2020-08-24)
Supplement: Supplementary file 1 [file supp_content.tex]

% \section*{Overview}

We outline this supplementary material as follows:
% \vspace{-3mm}
\begin{enumerate}
\item We show additional visual comparisons with competing baseline methods.
\item We describe the network configuration of the proposed model. The source code and the pre-trained model will be made available to fully reproduce our results in the paper and the supplementary material.
\item We provide implementation details, including training and testing procedures, as well as the implementation of baseline methods.
\item We present runtime analysis and the limitation of our method.
\end{enumerate}
% \vspace{-2mm}
%The source code and the pre-trained model will be made available to fully reproduce our results in the paper and the supplementary material.
% \noindent{We will release the source code and trained model file to simulate future research.}

%In this supplementary material, we present additional visual results and implementation details to complement the main manuscript.
%
%\begin{enumerate}
%    \item We provide additional visual results.
%    \item We provide the network architecture details of the proposed framework.
%    \item We describe the training details of our image/disparity generator.
%    \item We describe the training details of our MPI predictor.
%    \item We describe the testing details on NYU and RealEstate datasets.
%    \item We present the details of baseline methods.
%    \item We present the details of dis-occlusion handling methods.
%    \item We present the runtime analysis of our method.
    %\item We present the limitation of our method.
    %\item We present the additional details.
%\end{enumerate}
%
%We will release the source code, pre-trained model to facilitate future research.

\section{Additional visual results}
We present additional qualitative results in the attached HTML webpage.
Please refer to the file \href{main.html}{main.html}.
Our visual results consist of three main components.

\topic{(1) Visual Comparison}: We compare the novel view videos synthesized by our method and other baseline methods on the ADE20K~\cite{ade}, ADE20K-outdoor, NYU~\cite{nyu} datasets.
We demonstrate these results in the \emph{Visual Comparison} webpage.

\topic{(2) Background inpainting}: 
We explore alternative methods for handling the dis-occluded regions when rendering the scene at novel views.
According to the disparity image, we render the novel view images by standard backward warping the synthesized color image.
We then fill the missing pixels using different existing in-painting methods.
We experiment with the following three methods.
First, we apply simple diffusion-based inpainting for each frame independently. 
Second, we apply a learning-based image inpainting model (GatedConv)~\cite{gate} to fill in the dis-occluded regions independently for each frame.
Third, we use the 3D Ken Burns~\cite{ken}. The 3D Ken Burns method inpaints only one single view and may reveal additional dis-occluded regions in other views.
The results are shown in the \emph{Background inpainting} webpage.

\topic{(3) Number of depth layers in MPI:} We present the visual results of using a different number of depth layers (32, 64, 128) in our Multi-plane Image representation in the \emph{Number of depth layers} webpage.

\section{Network architecture}

%\topic{MPI generator.}
We provide the detailed network architectures of our two-stream image/disparity generator in \figref{arch}. 
We adopt the design from stereo magnification \cite{stereomag} for the MPI generator, which can be found in Table 1 in \cite{stereomag}.
%The MPI generator is following the design of Zhou~\etal~\cite{stereomag}, which can be found in Table 1 in \cite{stereomag}.

\begin{figure*}[h!]
\centering
\includegraphics[width=0.6\linewidth]{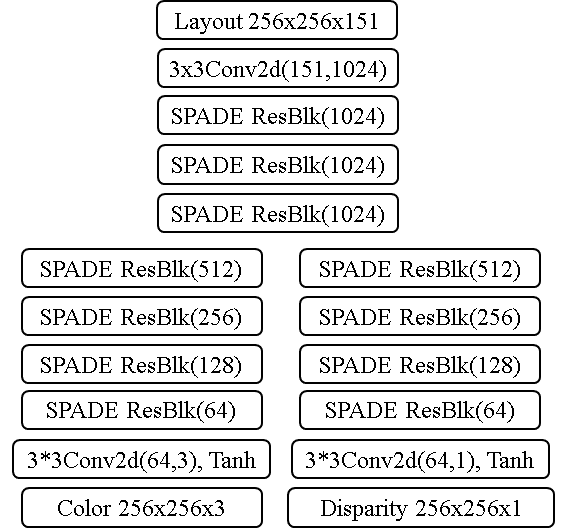}
\caption{\textbf{Network Architecture of image/disparity generator.} We modify the SPADE model~\cite{spade} to a two-stream color/disparity generators. One stream serves as the \emph{color generator}, while the other one is the \emph{disparity} generator. The two-stream generators share the first three SPADE-style ResNet blocks.
}
\label{fig:arch}
\end{figure*}

\section{Training}

\Paragraph{Image/disparity generator.}
\label{sec:fg}
Our training triple for image/disparity generator consists of a semantic layout, a color image, and a disparity image.
The semantic layout is a 2D one-hot representation of 151 classes in ADE20K~\cite{ade} dataset.
We generate the (pseudo) ground truth disparity image by the pretrained MiDaS~\cite{midas} predictor.
Since the disparity maps predicted by MiDaS are \emph{relative} prediction with unknown scale and shift, we further use the prediction from DPSNet~\cite{dpsnet} to transform the relative disparity map into \emph{absolute} disparity. 
Specifically, for each frame in RealEstate10K, we feed a stereo pair of images with the corresponding camera intrinsic value, and the camera poses to the DPSNet. 
The DPSNet predicts the absolute disparity map.
For each frame, we calculate the scaling and shifting transformation parameters between the MiDaS depth prediction and the DPSNet depth prediction values, and transform the MiDaS prediction to the absolute disparity image as our target disparity.
Following DPSNet, the disparity image has a range of 0 to 1, representing the disparity value from 1/2 to 32 equidistantly distributed.

We use a sequential training procedure for the image/disparity generator. %
The training consists of two steps: 
(a) semantic image synthesis: we first train the shared blocks and the color stream to generate the color image from the semantic layout; 
(b) semantic disparity synthesis: we then fix the shared blocks and the color stream, and only train the disparity stream, to generate the disparity image based on the semantic layout.
For (a) semantic image synthesis, we borrow the pretrained model of~\cite{spade}. 
The network is trained by 20,000 layout/image tuples in the ADE20K training set, optimized by Adam optimizer for 200 epochs with a learning rate of 0.0001 and the batch size of 32. 
The training losses include a VGG loss of weight 10, a GAN feature matching loss of weights 10 and a GAN loss of weight 1.
For (b) semantic disparity synthesis, we train the network using 150,000 layout/disparity tuples sampled from the RealEstate10K dataset. 
We use Adam optimizer to train the network with a $L_1$ loss, 150,000 iterations with a learning rate of 0.0002 and the batch size of 1.

\Paragraph{MPI predictor.}
%\section{Details of our MPI predictor}
The MPI predictor takes the source view image and the source view disparity as input, and predicts the MPI, which is then projected to novel views.
Our training pair for MPI predictor consists of two images with camera poses sampling from the videos of the RealEstate10K dataset~\cite{stereomag}. 
We follow the sampling method in \cite{stereomag}.
We first randomly sample an interval value from 1 to 10, then we sample a 10-frame sequence with the interval value. 
Finally, we randomly sample 2 frames from the sequence as our training pair
and the source view disparity is the same as \secref{fg}.
We use Adam optimizer to train the network with a $L_1$ loss for 150,000 iterations with a learning rate of 0.0002 and the batch size of 1.
Our MPI representation consists of 128 depth planes with the depth equally distributed from 1m to 100m according to inverse depth. 
We discretize the source view disparity to generate the alpha images based on the same depth values.

\section{Testing}
%\section{Details of testing}
\Paragraph{NYU dataset.}
As we train our model using the semantic classes from the ADE20K dataset, we are interested in validating how well the model generalizes to different semantic layouts.
We produce the testing results on the NYU dataset by mapping the classes of NYU to the classes of ADE. 
Each class is mapped to the class that has the same class name.
For the ``objects" class in NYU, we map it to the ``box" class in the ADE20K dataset.

\Paragraph{RealEstate dataset.}
We test our model using the testing videos in RealEstate10K \cite{stereomag} dataset. 
We use a semantic segmentation network PSPNet \cite{pspnet} pretrained on the ADE20K \cite{ade} dataset to obtain the testing semantic layout from the images. 
The results are shown in Figure 1 in the main paper.

\section{Baseline Approaches}

\Paragraph{Direct (U-Net).}
The model takes the 151-class semantic layout as input, and predicts a 72-layer MPI. 
The network is following the same U-Net in Zhou~\etal~\cite{stereomag}. 
We use Adam optimizer to train the network with a $L_1$ loss, 300,000 iterations, learning rate 0.0002, and batch size 1. 
The loss is applied between the projected novel view $\hat x^n$ and the ground truth novel view $x^n$.

\Paragraph{Direct (SPADE).}
The model takes the 151-class semantic layout as input, and predicts a 72-layer MPI. 
The network follows the design of Park~\etal~\cite{spade}. 
We use Adam optimizer to train the network for 100,000 iterations, learning rate 0.0002, and batch size 1. 
We apply the loss between the projected novel view $\hat x^n$ and the ground truth novel view $x^n$.
Specifically, we apply the following loss terms, a hinge GAN loss of weight 1, a GAN feature matching loss of weight 10, a VGG perceptual loss of weight 10, and a KL divergence loss of weight 0.5, following \cite{spade}.
The main differences between the Direct (SPADE) method and the Direct (U-Net) method are the use of the more advanced generator and training losses for synthesizing photorealistic images.

\Paragraph{Cascade (MPI).}
First, we use the SPADE model~\cite{spade} to generate the color image using a 151-class semantic layout as input. We use the model architecture from SPADE~\cite{spade}. 
Second, we train an MPI generator that takes color images as input, and predicts a 128-layer MPI. The network is following the same U-Net in Zhou~\etal~\cite{stereomag}. 
We use Adam optimizer to train the network with a $L_1$ loss, 100,000 iterations, learning rate 0.0002, and batch size 1.
We apply the loss between the projected novel view $\hat x^n$ and the ground truth novel view $x^n$.

\Paragraph{Cascade (KB).}
We use the SPADE model~\cite{spade} to generate the color image using a 151-class semantic layout as input. We then apply the model provided by Niklaus~\etal~\cite{ken}.

\Paragraph{Difference between the MPI.}
Note that the MPIs used in Direct (U-Net), Direct (SPADE), Cascade (MPI) and our model have different settings.
Direct (U-Net) and Direct (SPADE) predicts $x^s_{FG}$, $x^s_{BG}$, $\{w^s\}$ and $\{\alpha^s\}$.
Cascade (MPI) predicts $x^s_{BG}$, $\{w^s\}$ and $\{\alpha^s\}$, directly using the $x^s_{FG}$ generated by SPADE~\cite{spade}.
Our model only predicts $x^s_{BG}$ and $\{w^s\}$, directly using the $x^s_{FG}$ and $d^s$ as $\{\alpha^s\}$ generated by our two-stream image/disparity generator.

\Paragraph{Dis-occlusion handling baselines.}
We explore alternative methods for handling the dis-occluded regions when rendering at novel views. 
We applied standard backward warping to project $\hat x^s_{FG}$ by $\hat d^s$ to the novel view. We then apply Diffusion or GatedConv for inpainting the missing pixels at novel views.
For better visual quality, we apply a median filter with window size 19 to the disparity image $\hat d^s$. 
We also set the threshold on the occlusion mask so that a pixel is visible if half of the adjacent pixels are visible in a window of 9.

\section{Runtime analysis}
In Table \ref{tab:runtime}, we show the comparison of the training time, the inference time, and the rendering time of our model, conducted on a desktop equipped with NVIDIA GTX1080 and Xeon E5-2603 CPU cores.% @ 1.80GHz. 

\begin{table}[h!]\setlength{\tabcolsep}{5pt}
    \centering\scriptsize
    \caption{Run-time analysis.}\label{tab:runtime}
    \begin{tabular}{l|c}
        \toprule
        Training time of disparity generator (seconds / per iteration)         & 0.283 \\
        Training time of MPI generator (seconds / per iteration)         & 0.949 \\
        Inference time of image and disparity (seconds / per scene) & 0.040 \\
        Inference time of MPI (seconds / per scene)                 & 9.125 \\
        Rendering time of novel view (seconds / per view)                  & 0.443 \\
        \bottomrule
    \end{tabular}
\end{table}

\section{Failure Cases}
Our method sometimes may generate unnatural disparity maps, which result in implausible novel view rendering. 
\figref{failure} (top) shows the incorrect generated disparity map and \figref{failure} (middle) shows the corresponding generated color image.
Our method may also fail due to the incorrect MPI generation (e.g., generate incorrect disoccluded contents).
\figref{failure} (bottm) shows that novel view reveals clear visual artifacts.

\begin{figure}[h!]
\begin{center}
    \centering

    \mpage{0.22}{\includegraphics[width=\linewidth, height=\linewidth]{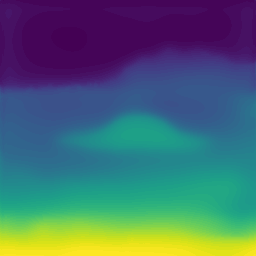}} 
    \mpage{0.22}{\includegraphics[width=\linewidth, height=\linewidth]{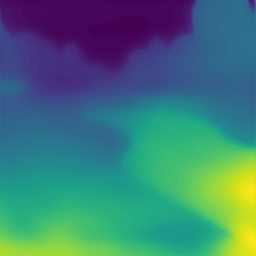}} 
    \mpage{0.22}{\includegraphics[width=\linewidth, height=\linewidth]{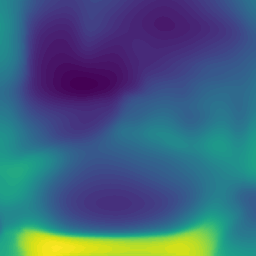}} \\
    
    %\vspace{0.5mm}
    \mpage{0.22}{\includegraphics[width=\linewidth, height=\linewidth]{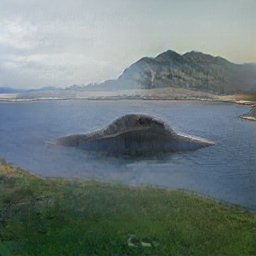}} 
    \mpage{0.22}{\includegraphics[width=\linewidth, height=\linewidth]{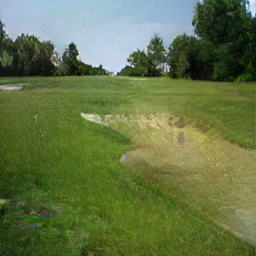}} 
    \mpage{0.22}{\includegraphics[width=\linewidth, height=\linewidth]{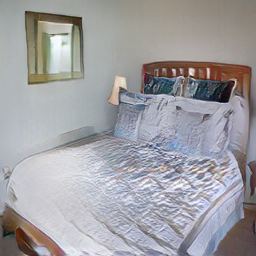}} \\
    
    %\vspace{0.5mm}
    \mpage{0.22}{\includegraphics[width=\linewidth, height=\linewidth,clip,trim={10px 0 0 0}]{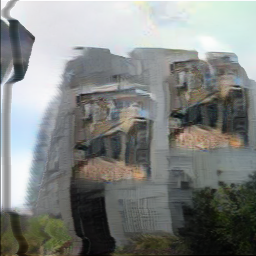}} 
    \mpage{0.22}{\includegraphics[width=\linewidth, height=\linewidth,clip,trim={10px 0 0 0}]{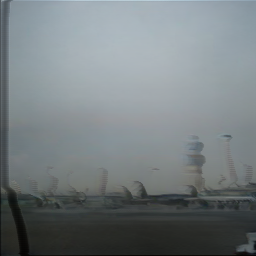}} 
    \mpage{0.22}{\includegraphics[width=\linewidth, height=\linewidth,clip,trim={10px 0 0 0}]{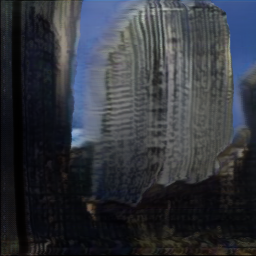}} \\
    
    %\vspace{0.5mm}
    \captionof{figure}{\textbf{Failure Cases.} (a) Our method generates unnatural disparity map \emph{(top, middle)}. (b) Our method generates incorrect disoccluded contents \emph{(bottom)}. }
    \label{fig:failure}
\end{center}
\end{figure}
